# Supplementary material for: Variability Matters : Evaluating inter-rater variability in histopathology for robust cell detection
Source: arXiv:2210.05175 source file (2022-10-11)
Supplement: Supplementary file 1 [file supplementary.tex]

\section{Supplementary Material}

\begin{figure}[!t]
\centering
    \includegraphics[width=0.99\textwidth]{drawable/cells1.pdf}
    
    \caption{Kappa=0.0034
    }
    \label{fig:varianceexample}
\end{figure} 
\begin{figure}[!t]
\centering
    \includegraphics[width=0.99\textwidth]{drawable/cells2.pdf}
    
    \caption{Kappa=0.13
    }
    \label{fig:varianceexample}
\end{figure} 

\begin{figure}[!t]
\centering
    \includegraphics[width=0.99\textwidth]{drawable/cells3.pdf}
    
    \caption{Kappa=0.42
    }
    \label{fig:varianceexample}
\end{figure} 
\begin{figure}[!t]
\centering
    \includegraphics[width=0.99\textwidth]{drawable/cells4.pdf}
    
    \caption{Kappa=0.43
    }
    \label{fig:varianceexample}
\end{figure} 

\begin{figure}[!t]
\centering
    \includegraphics[width=0.99\textwidth]{drawable/cells5.pdf}
    
    \caption{Kappa=0.80
    }
    \label{fig:varianceexample}
\end{figure} 

\begin{figure}[!t]
\centering
    \includegraphics[width=0.99\textwidth]{drawable/cells6.pdf}
    
    \caption{Kappa=0.86
    }
    \label{fig:varianceexample}
\end{figure}
